# Supplementary material for: Probabilistic Robustness in the Gap Metric
Source: arXiv:2507.10010 source file (2025-07-20)
Supplement: Supplementary file 1 [file appendix.tex]

\section*{Appendix}
